# Supplementary material for: Not Just Streaks: Towards Ground Truth for Single Image Deraining
Source: arXiv:2206.10779 source file (2024-07-29)

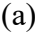

Supplement: Supplementary file 1 [file a.pdf]
