# Supplementary material for: Not Just Streaks: Towards Ground Truth for Single Image Deraining
Source: arXiv:2206.10779 source file (2024-07-29)
Supplement: Supplementary file 2 [file b.pdf]

OB
